# Supplementary material for: Quantitative understanding of negative thermal expansion in scandium trifluoride from neutron total scattering measurements
Source: arXiv:1905.09250 ancillary file (2020-07-24)
Supplement: Supplementary file 1 [file ScF3_SI_version3.pdf]

# A real-space experimental model for negative thermal expansion in scandium trifluoride: Electronic supplementary information

Martin T Dove*
*School of Physical Science and Technology, Sichuan University,*
*Chengdu 610065, People's Republic of China,*
*and School of Physics and Astronomy, Queen Mary University of London,*
*Mile End Road, London, E1 4NS, UK*

Juan Du and Anthony E Phillips
*School of Physics and Astronomy, Queen Mary University of London,*
*Mile End Road, London, E1 4NS, UK*

David A Keen
*ISIS Facility, Rutherford Appleton Laboratory,*
*Harwell Campus, Didcot, Oxfordshire, OX11 0QX, UK*

Matthew G Tucker
*Oak Ridge National Laboratory, Neutron Scattering Division,*
*1 Bethel Valley Road, Oak Ridge, TN 37831, USA*

## S1. RIETVELD REFINEMENT

Rietveld refinement was performed using the original GSAS package[1] with the ExpGUI interface[2]. Backgrounds were fitted using the standard approach based on Chebychev polynomials. We used GSAS Type 3 line shape as described in the manual[1]. We found, as is not uncommon with high-precision data, some difference in the refined values of the lattice parameters for data obtained using the cryostat and furnace, which is associated with the fact that the position of the sample is not identical in both sets of measurements. Therefore we did a self-calibration based on room temperature data, where we used the refined value of the lattice parameter from one set of data to allow refinement of a sample-displacement parameter with fixed lattice parameter in the other set of data, and which was therefore used for all data sets onwards.

One example of the quality of fitting is shown in Figure S1 for one detector bank.

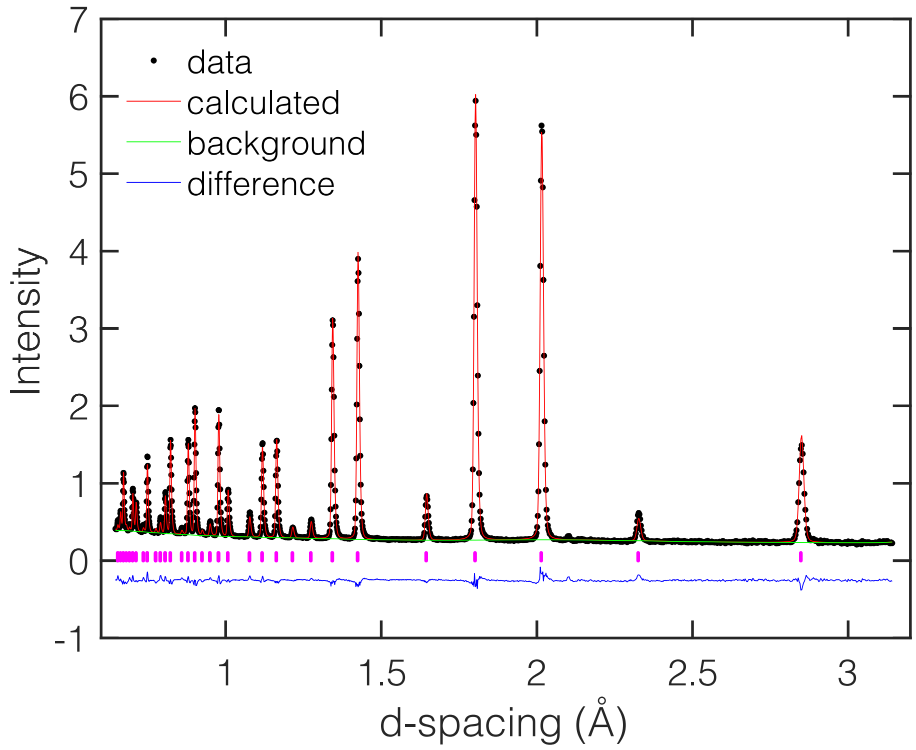


FIG. S1. Comparison of experimental (black filled circles) and model (red curve) diffraction patterns at a temperature of 10 K, with the difference shown as the blue curve and the fitted background as the green curve.

| $T$ (K) | $a$ (Å) | Sc $100 \times U_{\mathrm{iso}}$ (Å$^2$) | F $100 \times U_{11}$ (Å$^2$) | F $100 \times U_{22}$ (Å$^2$) | $R_{\mathrm{wp}}$ (%) | $R_{\mathrm{p}}$ (%) |
|---|---|---|---|---|---|---|
| 10 | 4.02777(15) | 0.55(3) | −0.21(6) | 0.52(4) | 3.1 | 3.1 |
| 100 | 4.02367(13) | 0.58(3) | −0.21(6) | 1.02(4) | 3.3 | 3.1 |
| 200 | 4.01941(21) | 0.75(4) | −0.24(7) | 1.77(5) | 3.1 | 3.0 |
| 290 | 4.01215(13) | 1.00(2) | −0.02(4) | 2.58(3) | 2.5 | 3.1 |
| 400 | 4.01047(15) | 1.19(2) | 0.05(5) | 3.45(4) | 2.4 | 2.9 |
| 500 | 4.00857(17) | 1.37(3) | 0.11(5) | 4.13(4) | 2.3 | 2.8 |
| 600 | 4.00713(24) | 1.49(3) | 0.02(6) | 4.75(5) | 2.4 | 2.9 |
| 700 | 4.00673(16) | 1.52(3) | 0.44(7) | 5.47(5) | 2.6 | 3.0 |
| 800 | 4.00560(20) | 1.84(3) | 0.41(6) | 6.16(5) | 2.3 | 2.7 |
| 950 | 4.00542(24) | 1.93(4) | 0.58(8) | 7.13(6) | 2.5 | 3.0 |
| 1000 | 4.00489(24) | 2.20(4) | 0.81(8) | 7.57(6) | 2.5 | 2.8 |
| 1100 | 4.00495(28) | 2.32(5) | 0.76(9) | 8.16(7) | 2.4 | 2.8 |
| 1200 | 4.00516(27) | 2.42(5) | 1.11(9) | 8.85(7) | 2.5 | 2.8 |

TABLE S1. Refined values of the cubic lattice parameter $a$ and the atomic displacement parameters (ADPs) from Rietveld refinement. Sc has fractional coordinations $0,0,0$ and F has fractional coordinates $\frac{1}{2},0,0$. By symmetry the ADP for Sc is isotropic, and for F $U_{22} = U_{33}$, and off-diagonal components are zero. Standard deviations on the last significant figures are given in brackets. The standard weight and profile $R$-factor values are given in the last two columns.

Refined values of the lattice parameters and atomic displacement parameters are given in Table S1. The temperature-dependence of the atomic displacement parameters are shown in Figure S2; the consistent linear variations with temperature indicates the quality of the refinements.

## S2. EQUATIONS FOR THE PAIR DISTRIBUTION FUNCTION

The scattering function is defined as

$$S(\mathbf{Q}) = \frac{1}{N} \sum_{j,k} \overline{b_j b_k} \left\langle \exp(i\mathbf{Q} \cdot \mathbf{r}_{jk}) \right\rangle \tag{S1}$$

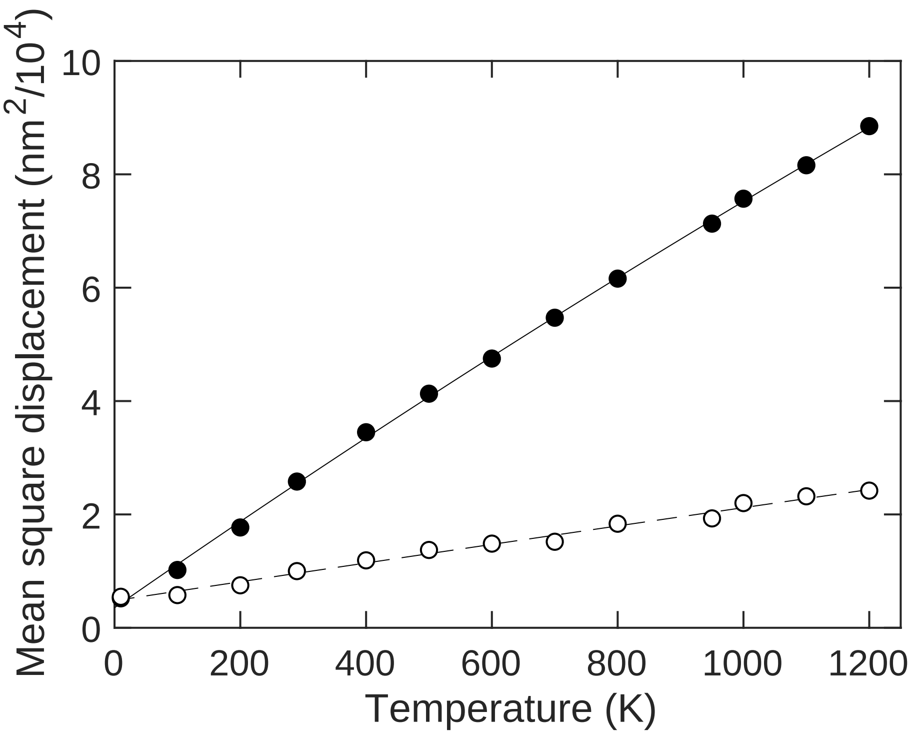


FIG. S2. Temperature dependence of the Sc isotropic atomic displacement parameter (open circle) and of the F $U_{22}$ parameter (filled circle), with the straight lines given as guides to the eye.

where the sum is over all pairs of atoms $j$ and $k$, $b_j$ is the scattering length of atom $j$, the overline and angle brackets denote averages, $\mathbf{r}_{jk}$ is the vector between atoms $j$ and $k$, and $\mathbf{Q}$ is the scattering vector defined as the difference between the incoming and scattered radiation wave vectors. The average is over all instances in time. Because experiments are performed on powdered samples and data are collected for many orientations of $\mathbf{Q}$ at fixed modulus $Q = |\mathbf{Q}|$, by averaging over all angles between $\mathbf{Q}$ and $\mathbf{r}$ we obtain

$$S(Q) = \frac{1}{N}\sum_j \overline{b_j^2} + \frac{1}{N}\sum_{j\neq k} \overline{b_j}\,\overline{b_k}\,\frac{\sin(Qr_{jk})}{Qr_{jk}} \tag{S2}$$

where we separate out the cases $j = k$ from $j \neq k$, and in the second term we express the fact for $j \neq k$, $\overline{b_j b_k} = \overline{b_j}\,\overline{b_k}$. We now drop the overbar in $\overline{b}$ for ease of writing. The first term in equation S2 is better represented as a sum over atom types rather than over all individual atoms:

$$\frac{1}{N}\sum_j \overline{b_j^2} = \sum_m c_m \overline{b_m^2} \tag{S3}$$

where $c_m$ is the concentration of atoms of type $m$. In the same spirit we can write the second term in equation S2 in terms of an integral over the distribution of distances between different atom types rather than as a sum over all atom pairs. We define the number of atoms of type $n$ lying within a spherical shell of thickness d$r$ at a distance $r$ from an atom of type $m$ as $4\pi r^2 \mathrm{d}r \times c_n\rho \times g_{mn}(r)$. Therefore the pair sum can be replaced by

$$\frac{1}{N}\sum_{j,k} b_j b_k \frac{\sin(Qr_{jk})}{Qr_{jk}} = 4\pi\rho \int \sum_{m,n} c_m c_n b_m b_n r^2 g_{mn}(r) \frac{\sin(Qr)}{Qr}\,\mathrm{d}r \tag{S4}$$

In the limit that $r \to \infty$, $g_{mn}(r) \to 1$, reflecting the fact that a shell of large radius will contain a more uniform sample of atoms. It is thus better to subtract this from the data, because it does no more than add a constant and a constant in a Fourier transform gives a delta function at $Q = 0$. Thus it is better to separate this out to give

$$i(Q) = S(Q) - \textstyle\sum_m c_m \overline{b_m^2} - S_0 = 4\pi\rho \displaystyle\int \sum_{m,n} c_m c_n b_m b_n r^2 \left(g_{mn}(r) - 1\right) \frac{\sin(Qr)}{Qr}\,\mathrm{d}r \tag{S5}$$

where $S_0$ is the delta function at $Q = 0$:

$$S_0 = 4\pi\rho \int \sum_{m,n} c_m c_n b_m b_n r^2 \frac{\sin(Qr)}{Qr}\,\mathrm{d}r \tag{S6}$$

We now define the pair distribution function

$$D(r) = 4\pi\rho r \sum_{m,n} c_m c_n b_m b_n \left(g_{mn}(r) - 1\right) \tag{S7}$$

With this definition we can rearrange equation S5 as

$$Qi(Q) = \int_0^\infty D(r)\sin(Qr)\,\mathrm{d}r \tag{S8}$$

This has the reverse transformation:

$$D(r) = \frac{2}{\pi}\int_0^\infty Qi(Q)\sin(Qr)\,\mathrm{d}r \tag{S9}$$

We consider $D(r)$ to be our PDF of choice to work with, because of its fundamental role as the Fourier transform of the data function $Qi(Q)$. As such, errors are to a first approximation spread uniformly across the spread of values of $r$ in $D(r)$.

We note that there are several formulations of the equations associated with the PDF and total scattering; several of these have been compared by one of the authors[3].

| $T$ (K) | F–F (Å) | F–Sc (Å) | Sc–Sc (Å) |
|---|---|---|---|
| 10 | 2.33–3.23 | 1.85–2.20 | 3.73–4.31 |
| 1200 | 2.11–3.61 | 1.74–2.38 | 3.55–4.49 |

TABLE S2. Distance windows used in RMC refinement, showing the values for the lowest and highest temperatures.

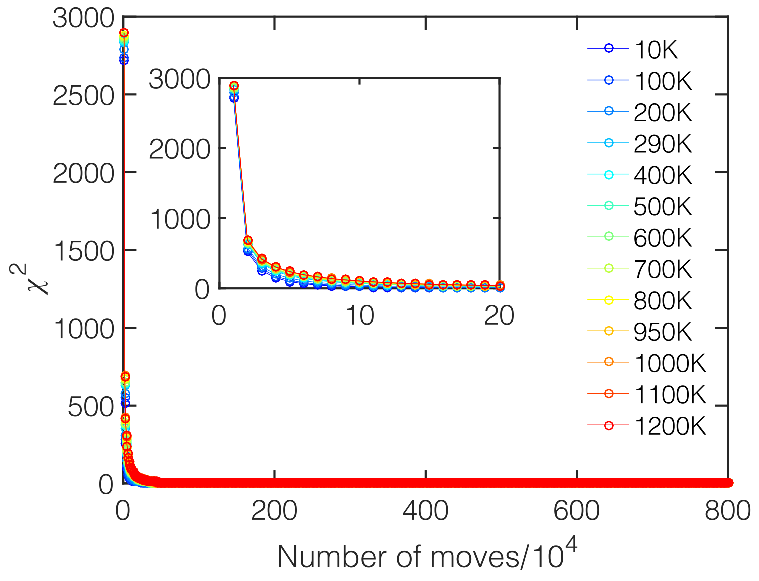


FIG. S3. Confirmation of the convergence of RMC refinement. The figure inside shows the details between 0 and 20 of the $x$ axis.

## S3. REVERSE MONTE CARLO METHOD

RMC simulations were performed using the RMCprofile code[4]. To reduce the risk of atoms moving from from their sites we used distance windows restraints for all nearest neighbour pairs. The windows were adjusted for temperature, with limiting cases given in Table S2. RMC agreement factors were based on the $i(Q)$ data (the data were convolved with a sinc function for comparison to account for the finite range in the RMC-calculated PDF data), the $D(r)$ data and the Bragg diffraction profile $y(t)$, where $t$ is the neutron

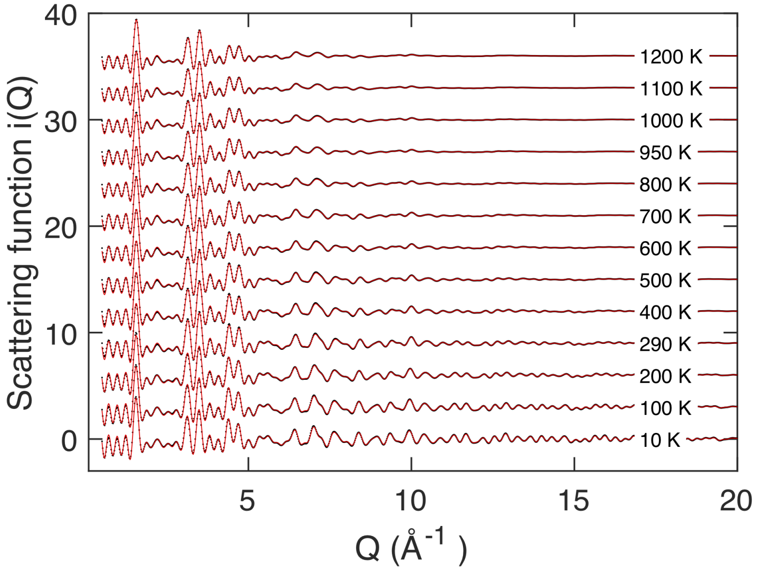


FIG. S4. Comparison of experimental and RMC-derived $i(Q)$ functions. Black lines are from the RMC calculation and red lines are the experimental data.

flight time. The RMC method uses a set of $\chi^2$ functions:

$$\chi^2 = \sigma_D^{-2} \sum_r \left(D_{\mathrm{exp}}(r) - D_{\mathrm{calc}}(r)\right)^2 + \sigma_i^{-2} \sum_r \left(i_{\mathrm{exp}}(Q) - i_{\mathrm{calc}}(Q)\right)^2 + \sigma_{\mathrm{B}}^{-2} \sum_r \left(y_{\mathrm{exp}}(t) - y_{\mathrm{calc}}(t)\right)^2 \quad \text{(S10)}$$

where the $\sigma$ values are a set of weighting parameters. The RMC method works by moving an atom chosen at random by a random displacement, and calculating the change in $\chi^2$. If the change $\Delta\chi^2$ is negative, the move is accepted, but if it is positive it is accepted with probability $\exp(-\Delta\chi^2/2)$. The RMC for each temperature was initially run until the value of $\chi^2$ reached a constant value, as shown in Figure S3, and thereafter run again to generate 10 independent configurations for subsequent analysis.

The quality of the RMC fit to the various data sets are show in Figures S4–S6 showing the $i(Q)$, $D(r)$ and Bragg profile data respectively. The high quality of the fitting is demonstrated in these figures.

The partial PDF functions $g(r)$ for Sc–Sc, Sc–F and F–F atom pairs are shown in Figures S7, S8 and S9 respectively.

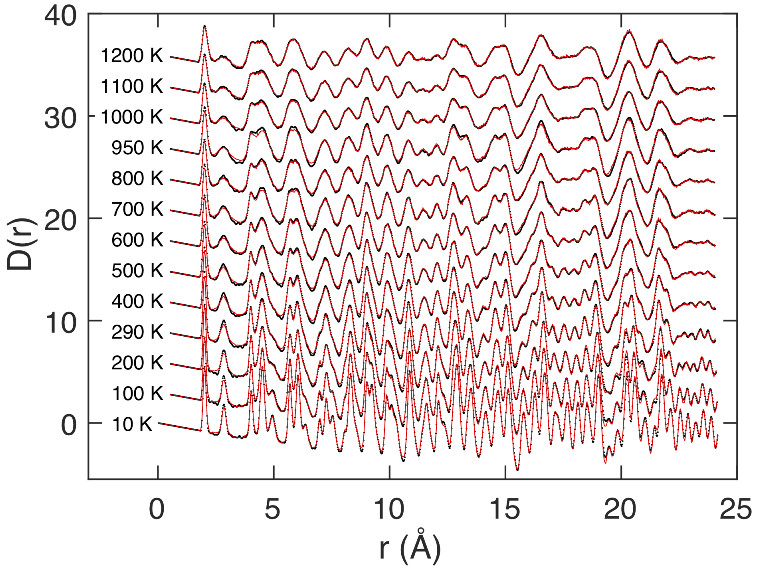


FIG. S5. Comparison of experimental and RMC-derived $D(r)$ functions. Black lines are from the RMC calculation and red lines are the experimental data.

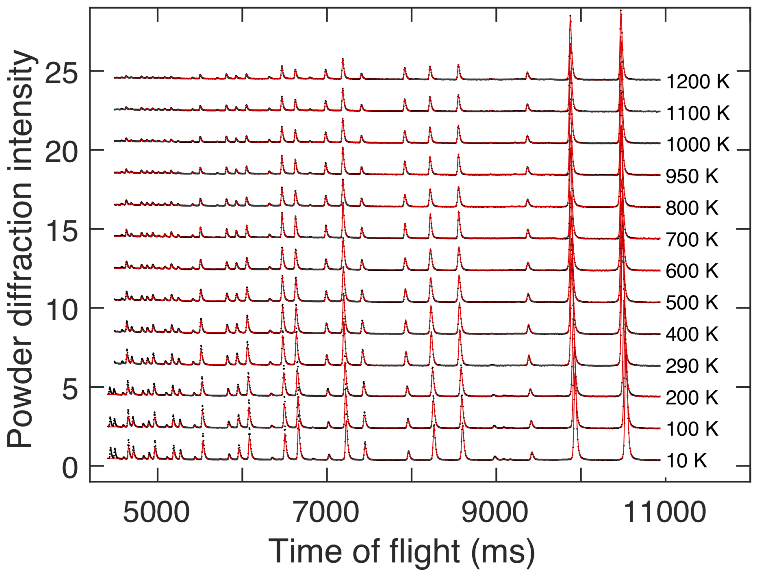


FIG. S6. Comparison of experimental and RMC-derived Bragg profile functions. Black lines are from the RMC calculation and red lines are the experimental data.

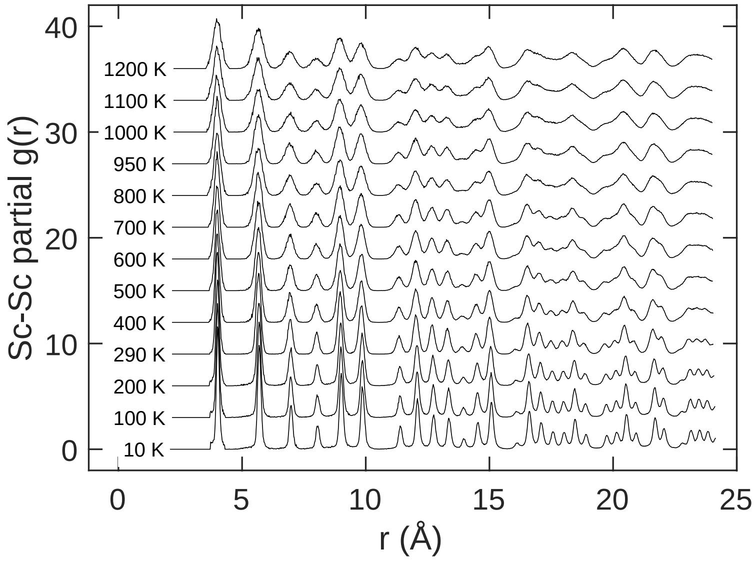


FIG. S7. Partial pair distribution function $g(r)$ for Sc–Sc atomic pairs.

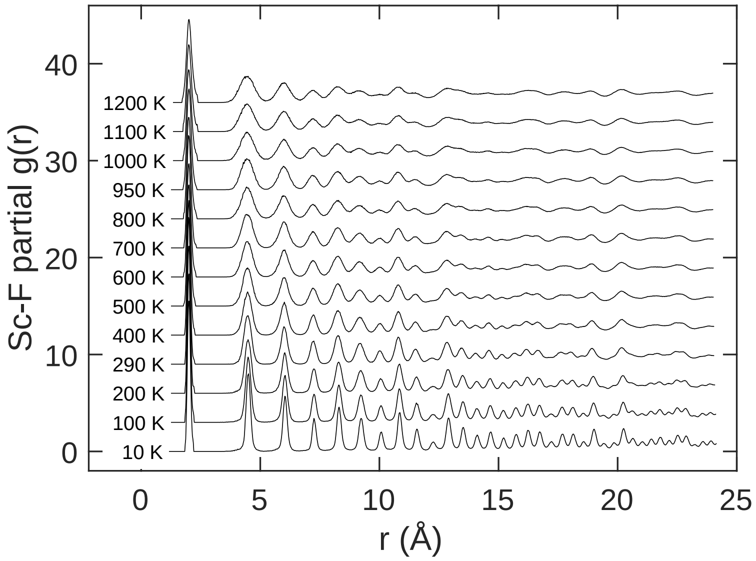


FIG. S8. Partial pair distribution function $g(r)$ for Sc–F atomic pairs.

## S4. FLEXIBILITY MODEL

We studied a model for $ScF_3$ in which we used only three potential energy functions and no electrostatic interactions. Calculations were performed using the GULP lattice energy and lattice dynamics code[6]. The three functions describe a) the stretching of the Sc–F bond, b) the bending of the F–Sc–F right-angle bond angle within the $ScF_6$ octahedron, and c)

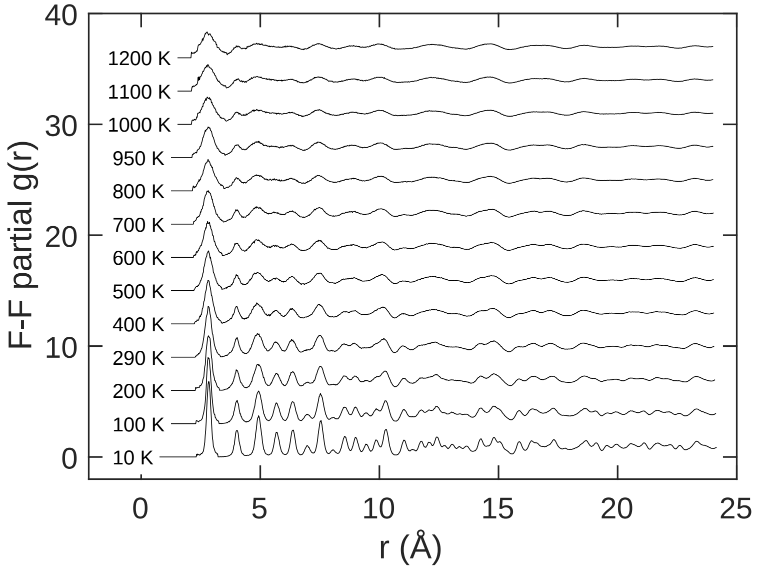


FIG. S9. Partial pair distribution function $g(r)$ for F–F atomic pairs.

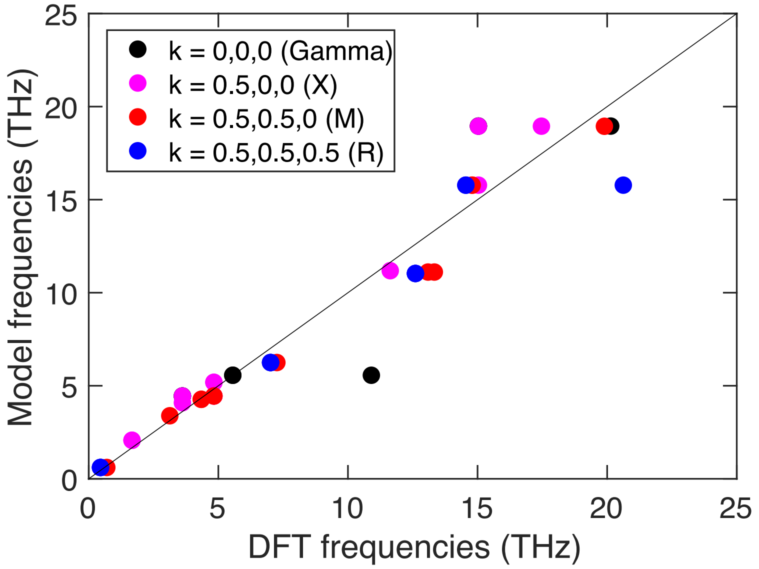


FIG. S10. Comparison of model and DFT phonon frequencies (from reference 5) for four wave vectors.

the bending of the linear Sc–F–Sc linkage. The Sc–F bond was described using a Morse potential of the form

$$E(r) = D\left(\exp\left(2\alpha(r_0 - r)\right) - 2\exp\left(\alpha(r_0 - r)\right)\right) \tag{S11}$$

with parameters $D = 2.0$ eV, $r_0 = 2.0125$ Å, and $\alpha = 1.55$ Å$^{-1}$, chosen to give the experimental bond length and to reproduce the highest frequency in the phonon dispersion curves as calculated by DFT.[5] The F–Sc–F angle potential is described by a simple quadratic function in the bond angle $\theta$:

$$E(\theta) = \frac{1}{2}k\,(\theta - \theta_0)^2 \tag{S12}$$

where $\theta_0 = 90°$. $k$ is the primary variable in the model, but in what follows below we start with the value $k = 1.5$ eV/rad designed to best reproduce the DFT phonon dispersion curves. The Sc–F–Sc angle potential is described using the function

$$E(\theta) = K\,(1 + \cos\theta) \tag{S13}$$

where $K = 0.025$ eV, tuned to reproduce the frequency of the RUM along the line $M$–$R$ in reciprocal space calculated by DFT. The calculated frequencies for four wave vectors are compared with the DFT values in Figure S10, showing reasonable agreement. The phonon dispersion curves calculated from this model are shown in Figure S11, where they are coloured according to the sign of the mode Grüneisen parameters obtained by calculations for two volumes using the method described in detail in reference 7. This model is too simple to expect excellent agreement with the DFT phonon dispersion curves – for example, there are several branches with completely flat dispersion across a line in reciprocal space, and the model calculated the elastic constants $C_{12} = 0$ – but it has given better agreement than might have been expected. In particular, the modes with negative Grüneisen parameters in the model are the same as those identified in the DFT study of reference 5.

This model has been use in a molecular dynamics simulation (using the program DL_POLY[8]) for a range of values of the F–Sc–F bending force constant $k$, and the results analysed using the program GASP[9–11] as described in the main text. We obtained the results shown in Figure S12, where we show the percentage of motion associated with octahedral rotations, bond-bending and bond-stretching for a range of values of the bond-bending force constant $k$. We used a temperature of 300 K, but in general the temperature appears not to matter too much because the motions reflect the harmonic phonon eigenvectors which do not change much with temperature within a quasi-harmonic approximation. The important results are

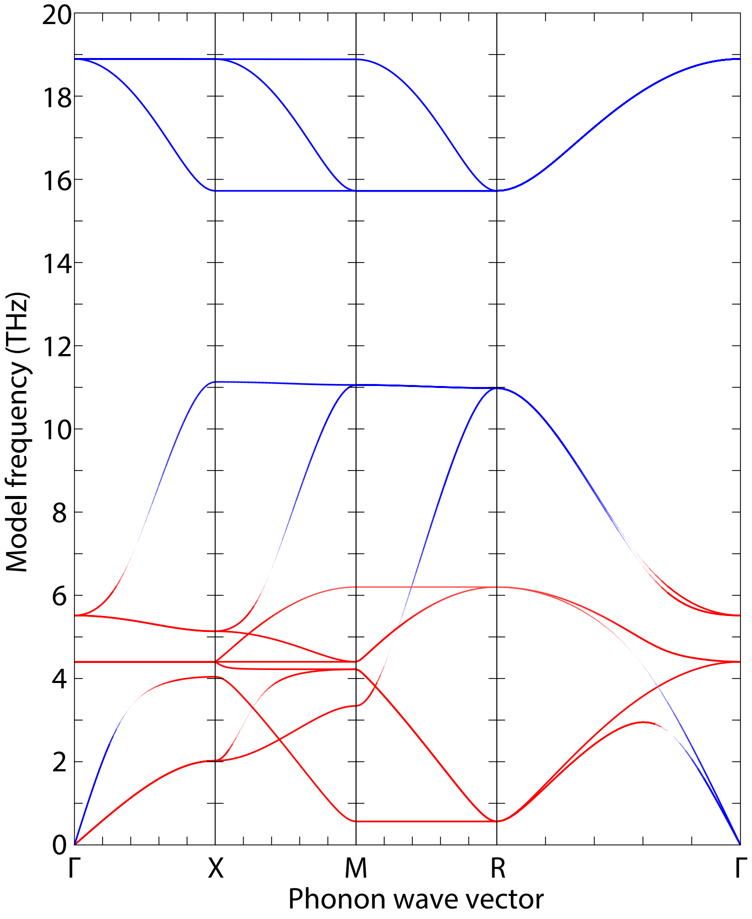


FIG. S11. Calculated dispersion curves for the simple model described in the text. Red curves are those with negative Grüneisen parameters and blue curves are those with positive Grüneisen parameters. The special points in reciprocal space are $\Gamma = (0,0,0)$, $\mathrm{X} = (\frac{1}{2},0,0)$, $\mathrm{M} = (\frac{1}{2},\frac{1}{2},0)$ and $\mathrm{R} = (\frac{1}{2},\frac{1}{2},\frac{1}{2})$.

1. When $k = 0$ some of the motion is interpreted by GASP as corresponding to rotational motion. This reflects the fact that if bonds are free to rotate to the left or right, there will be cases where they move as if a rotation by chance.

2. As $k$ gets larger, the proportion of octahedral rotation increases and the proportion of bending decreases. However, as $k$ increases the rate of change of these two proportions with $k$ becomes progressively smaller, so that at high $k$ these two proportions are roughly similar. We noted in the main text that the number of RUMs that will give rise to rotations is infinitesimally small which will require there always to be a

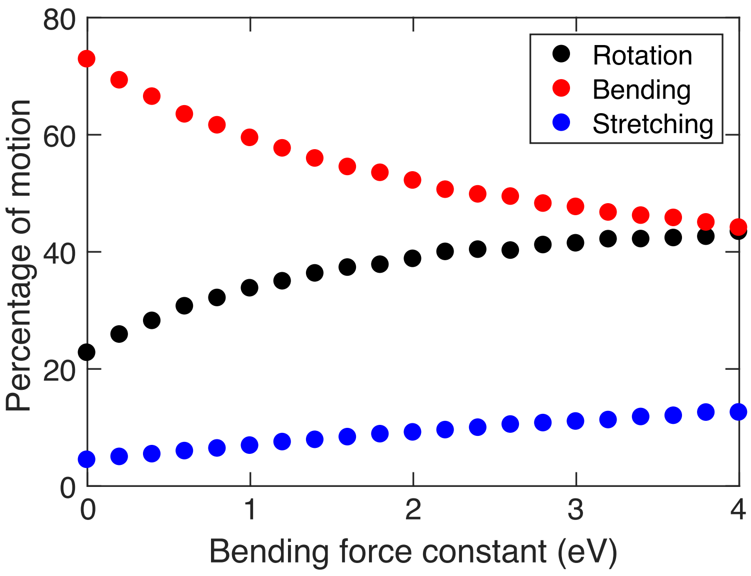


FIG. S12. GASP model.

significant amount of bond bending.

3. With increasing $k$ the proportion of bond-stretching appears to increase. This does not imply an increase in bond stretching per se, because as a proportion of the total motion it is a reflection of the high energy and hence lower amplitude of bond-bending motions.

As we note in the main text, the case of $ScF_3$ will be at the lower-$k$ end of this diagram. On the other hand, the case of $SrTiO_3$, with which we make some comparison, is for higher $k$[12]. This is actually reflected in the insight gained by comparison of the acoustic modes along the $[1, 0, 0]$ direction in both materials. The ratio of the frequencies of the longitudinal and transverse acoustic modes at small wave vector in this direction, which is given as $\mathcal{R} = \sqrt{C_{11}/C_{44}}$, where $C_{11}$ is the tensile elastic constant and $C_{44}$ is the shear elastic constant. In the case of $SrTiO_3$, the value of $\mathcal{R}$ from neutron scattering measurements[13] is around 2, but in the case of $ScF_3$ the value from DFT calculations is around 4. This is consistent with the GASP results for $ScF_3$ and $SrTiO_3$ given in the paper, with the effective $k$ for $ScF_3$ at the low end of the $k$ range spanned in Figure S12, and the effective $k$ for SrTiO $_3$ being at the high end of the $k$ range. It is not meaningful to ascribe an absolute number because the match is not perfect. For example, our lattice models for $ScF_3$ described above have value $k = 1.5$ eV/rad that is higher than we would expect from comparing Figure

S12 with experimental data. This is because of the over-simplification of the model, which is designed to be indicative rather than fully accurate.

---

* martin.dove@qmul.ac.uk

[1] A. C. Larson and R. B. V. Dreele, Los Alamos National Laboratory Report LAUR **86**, 748 (2001).

[2] B. H. Toby, Journal of Applied Crystallography **34**, 210 (2001).

[3] D. A. Keen, Journal of Applied Crystallography **34**, 172 (2001).

[4] M. G. Tucker, D. A. Keen, M. T. Dove, A. L. Goodwin, and Q. Hui, Journal of Physics: Condensed Matter **19**, 335218 (2007).

[5] C. W. Li, X. Tang, J. A. Muñoz, J. B. Keith, S. J. Tracy, D. L. Abernathy, and B. Fultz, Physical Review Letters **107**, 195504 (2011).

[6] J. D. Gale and A. L. Rohl, Molecular Simulation **29**, 291 (2003).

[7] L. H. N. Rimmer and M. T. Dove, Journal of Physics: Condensed Matter , 185401 (2015).

[8] I. T. Todorov, W. Smith, K. Trachenko, and M. T. Dove, Journal of Materials Chemistry **16**, 1911 (2006).

[9] S. A. Wells, M. T. Dove, and M. G. Tucker, Journal of Physics: Condensed Matter **14**, 4567 (2002).

[10] S. A. Wells, M. T. Dove, M. G. Tucker, and K. Trachenko, Journal of Physics: Condensed Matter **14**, 4645 (2002).

[11] S. A. Wells, M. T. Dove, and M. G. Tucker, Journal of Applied Crystallography **37**, 536 (2004).

[12] Q. Hui, M. G. Tucker, M. T. Dove, S. A. Wells, and D. A. Keen, Journal of Physics: Condensed Matter **17**, S111 (2005).

[13] W. G. Stirling, Journal of Physics C: Solid State Physics **5**, 2711 (2001).
